# Supplementary material for: Class-Prototype Conditional Diffusion Model with Gradient Projection for Continual Learning
Source: arXiv:2312.06710 source file (2024-03-21)
Supplement: Supplementary file 2 [file preamble.tex]

%
% --- inline annotations
%
\usepackage[dvipsnames]{xcolor}
\newcommand{\red}[1]{{\color{red}#1}}
\newcommand{\todo}[1]{{\color{red}#1}}
\newcommand{\TODO}[1]{\textbf{\color{red}[TODO: #1]}}
% --- disable by uncommenting  
% \renewcommand{\TODO}[1]{}
% \renewcommand{\todo}[1]{#1}
